# Supplementary material for: Light Dark Matter Search with a High-Resolution Athermal Phonon Detector Operated Above Ground
Source: arXiv:2007.14289 ancillary file (2021-10-12)
Supplement: Supplementary file 1 [file CPD_DM_Search_Data_Release.pdf]

# SuperCDMS Data Release for CPD DM Search

SuperCDMS Collaboration

This document accompanies the public data release for the SuperCDMS-CPD dark matter (DM) search carried out at the SLAC surface facility and gives explanatory material for the released files. The light DM search results can be found in Ref. [1]. The provided data allow the community to use this release to remake all figures in the paper, as well as analyze the unbinned energy spectrum within the DM search region-of-interest (ROI) of reconstructed energies below 240 eV.

## 1 Description of the Files

In the parent directory of the data release, there are two files (excluding this `.pdf` file) and four folders. Each folder is named `figure#`, where `#` is an integer from one to four, and contains multiple `.txt` files for recreating the figures from the paper. Before describing the contents of each folder, we describe the two files in the parent directory.

- `recon_energies_roi.txt`: This file contains the unbinned reconstructed event energies for each event in the DM ROI that passed the prepulse baseline cut and chi-square cut. In Fig. 2, the main plot shows a binned and signal efficiency-corrected spectrum, which can be recreated using this data.
- `cpd_data_release.ipynb`: This file is a Jupyter Notebook that contains code for reproducing each of the plots in the DM search paper, such that the reader does not have to start from scratch. This notebook uses the data files in each of the `figure#` folders, as described in the subsections below. To run the notebook using Jupyter, the notebook expects a Python 3 installation with NumPy and Matplotlib. There is an option to use  $\text{\TeX}$  for the plot text as well, but this is not necessary for the reproduction of the results.

### 1.1 Contents of `figure1` Folder

The contents of the `figure1` folder are four separate `.txt` files, each of which have two columns of comma-delimited data. Each of these files allows the creation of the plot shown in Fig. 1. In each data file for this figure, the x-values are saved in seconds, while the figure plots in milliseconds. The FPGA trigger threshold is a horizontal line at 11.77 ADC bins, corresponding to the black dotted line in Fig. 1.

- `rawpulse.txt`: This file contains the raw data corresponding to the gray line in Fig. 1. The file has two columns, where the first column is the x-values in units of seconds, and the second column is the y-values in units of ADC bins.
- `optimumfilter.txt`: This file contains the offline optimal filter (OF) result of the raw data, corresponding to the blue line in Fig. 1. The file has two columns, where the first column is the x-values in units of seconds, and the second column contains the y-values in units of ADC bins.

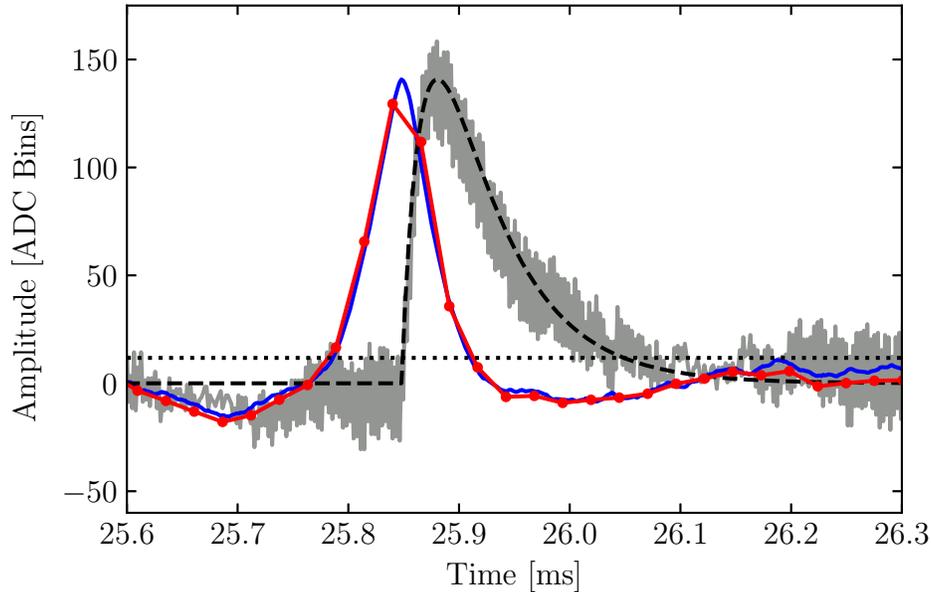

Figure 1: (Caption from Ref. [1]) A zoomed-in portion of an example event within the analysis ROI. The raw pulse (gray) is compared to the offline optimal filter result (blue), the pulse template scaled by the fit result (black dashed), the FPGA filter result (red with dots), and the FPGA trigger threshold (black dotted). The offline and FPGA optimal filters are highly correlated, but not exactly the same, with corresponding energy estimates for this event of 187 eV and 179 eV, respectively. The offset between the optimal filters and the raw pulse is an artifact of the filters, as they were set up to determine the time of the beginning of the pulse, as opposed to the maximum of the pulse.

- `fitresult.txt`: This file contains the pulse template scaled by the OF amplitude calculated from the offline OF algorithm, corresponding to the black dashed line in Fig. 1. The file has two columns, where the first column is the x-values in units of seconds, and the second column contains the y-values in units of ADC bins.
- `fpgafilter.txt`: This file contains the FPGA filter result of the raw data, corresponding to the red line with dots in Fig. 1. The file has two columns, where the first column is the x-values in units of seconds, and the second column contains the y-values in units of ADC bins.

## 1.2 Contents of figure2 Folder

The contents of the `figure2` folder are two separate `.txt` files, both of which have two columns of comma-delimited data. These files contain the two binned spectra shown in Fig. 2, each corresponding to a different energy estimator. The file `recon_energy_drde.txt` allows creation of the main plot of Fig. 2, while the file `e.etf_drde.txt` allows creation of the inset. Both spectra have been corrected for the cut efficiencies of the chi-square and baseline cuts, but not the trigger efficiency (as this is contained within convolution with a bivariate probability density function). For the vertical lines in the inset, these values are set at (in order of increasing energy in keV):

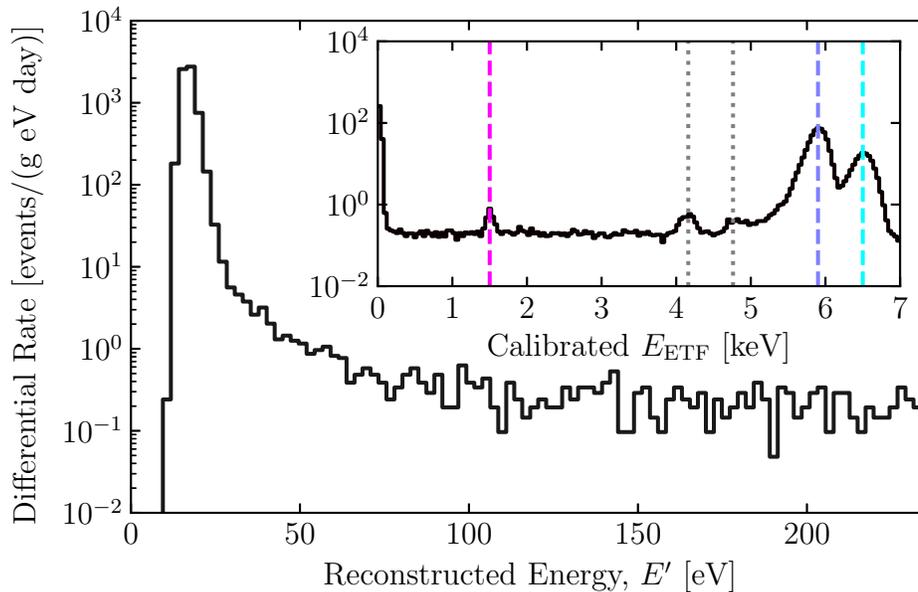

Figure 2: (Caption from Ref. [1]) Measured energy spectrum in the DM-search ROI for the full exposure after application of the quality cuts. The data have been normalized to events per gram per day per eV and have been corrected for the event-selection efficiency, but not the trigger efficiency. The inset shows the calibrated  $E_{\text{ETF}}$  spectrum up to 7 keV, noting the locations of the different spectral peaks. The known values of the dashed lines are 1.5, 5.9, and 6.5 keV for the Al fluorescence (pink),  $^{55}\text{Fe}$   $K_{\alpha}$  (blue), and  $^{55}\text{Fe}$   $K_{\beta}$  (cyan) lines, respectively. The two dotted gray lines between 4 and 5 keV in calibrated  $E_{\text{ETF}}$  are the Si escape peaks [2].

1.5, 4.161, 4.761, 5.9, and 6.5. Note that, taking into account the exposure and the total signal efficiency, the previously-discussed unbinned spectrum file `recon_energies_roi.txt` can also be used to recreate the histogram in the main plot of this figure.

- `recon_energy_drde.txt`: This file contains the binned DM ROI spectrum for the OF-based reconstructed energy used to set the DM exclusion limit. The first column is the reconstructed energy in units of eV, and the second column is the differential rate ( $\partial R/\partial E$ ) in units of events/g/eV/day. These values correspond to the bin centers of the reconstructed energy spectrum in the main plot of Fig. 2.
- `e_etf_drde.txt`: This file contains the energy spectrum for the calibrated integral energy estimator ( $E_{\text{ETF}}$ ). The first column is the calibrated  $E_{\text{ETF}}$  in units of keV, and the second column is the differential rate ( $\partial R/\partial E$ ) in units of events/g/eV/day. These values correspond to the bin centers of the spectrum in the inset of Fig. 2. Because this is a different energy estimator with a worse baseline energy resolution than the OF-based reconstructed energy estimator, these values cannot be used to recreate the main plot of this figure.

### 1.3 Contents of figure3 Folder

The contents of the `figure3` folder consist of a single comma-delimited file, which contains the limit result reported in the paper. This data release only includes the SuperCDMS-CPD limit, as

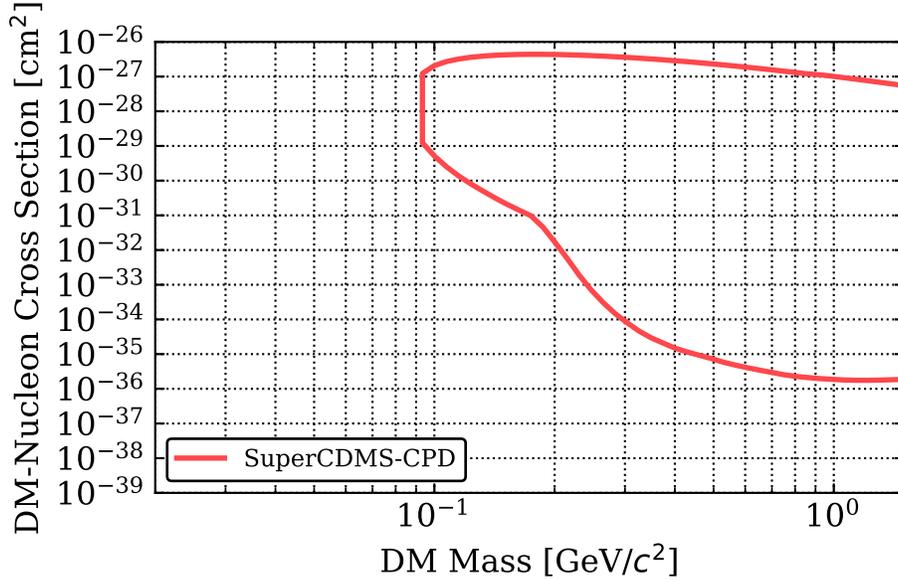

Figure 3: (Caption excerpt from Fig. 3 of Ref. [1]) The 90% C.L. limits on the spin-independent DM-nucleon cross section as a function of DM mass for this work.

shown in Fig. 3. We direct the reader to the references in Ref. [1] for the other DM limits shown in the corresponding figure in the paper. We also note that the data provided in this release are not enough to fully reproduce the limit shown in Fig. 3. The spectra provided for Fig. 4 do not account for the full range of masses (specifically, DM masses higher than about  $400 \text{ MeV}/c^2$ ), and correspond to the signal models calculated from a single pulse simulation. Furthermore, the spectra used for the upper edge of the limit have not been provided. If more data is needed for reproduction of these results, we recommend contacting the authors of the paper.

- `cpd_limit.txt`: This file contains the limit result reported in the paper. The first column is the DM mass in units of  $\text{GeV}/c^2$ , and the second column is the DM-nucleon cross section in units of  $\text{cm}^2$ .

#### 1.4 Contents of figure4 Folder

The contents of the `figure4` folder are 14 separate comma-delimited `.txt` files, which provide the data needed to create Fig. 4. The explanation of each file is below. Each of the spectra provided in this folder have been normalized by the cut efficiencies on the DM search data.

- `recon_energies_low_drde.txt`: This file contains the binned reconstructed energy spectrum normalized to units of  $\text{events}/\text{g}/\text{eV}/\text{day}$ . The first column is the reconstructed energy in units of  $\text{eV}$ , and the second column is the differential rate ( $\partial R/\partial E$ ) in units of  $\text{events}/\text{g}/\text{eV}/\text{day}$ . These values correspond to the bin centers reconstructed energy spectrum in Fig. 4. Note that the energies do not go above  $40 \text{ eV}$ , as this is the upper x-limit of the plot.
- `oi_drde_mass_###_cs_X.XXe-XX.txt`: There are 13 distinct files with names of this form. In the file name, `###` corresponds to the DM mass in units of  $\text{MeV}/c^2$ , and `X.XXe-XX` corresponds

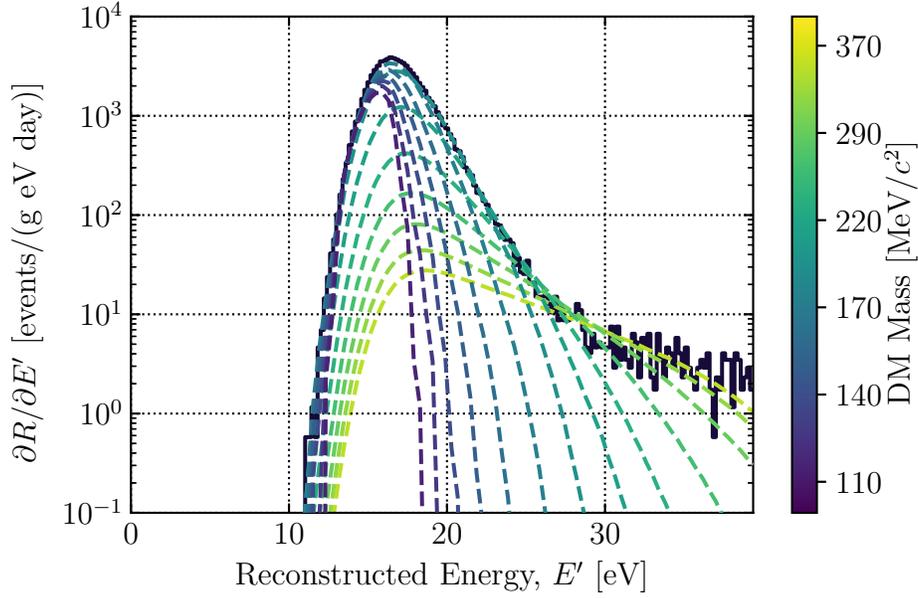

Figure 4: (Caption from Ref. [1]) The event spectrum for the DM search data below 40 eV in reconstructed energy. The data have been normalized to events per gram per day per eV and have been corrected for the signal efficiency of the data-quality cuts, but not the confidence ellipse and trigger time cuts. The colored dashed lines represent the calculated event rates for selected DM cross sections and masses from the 90% C.L. OI limit for a single pulse simulation, where the optimum intervals in recoil energy are below 40 eV. Sensitivity to DM masses below  $400 \text{ MeV}/c^2$  corresponds to recoil energies below 40 eV, with the lowest masses requiring energy sensitivity down to about 15 eV.

to the DM-nucleon cross section in scientific notation in units of  $\text{cm}^2$ . These files correspond to the dashed lines in Fig. 4, which represent the signal models that correspond to each DM mass and DM-nucleon cross section chosen by the optimum interval code for an example simulation. Note that the mass and cross section values may not exactly match the provided limit for Fig. 3, as the limit is the result of taking the median of eight simulations. In each of these files, the first column is the reconstructed energy in units of eV, and the second column is the differential rate ( $\partial R/\partial E$ ) in units of events/g/eV/day.

## References

- [1] I. Alkhatib *et al.* (SuperCDMS Collaboration), Light Dark Matter Search with a High-Resolution Athermal Phonon Detector Operated above Ground. *Phys. Rev. Lett.* **127** (2021). arXiv: 2007.14289 [hep-ex].
- [2] S. J. B. Reed and N. G. Ware. Escape peaks and internal fluorescence in X-ray spectra recorded with lithium drifted silicon detectors. *J. Phys. E Sci. Instrum.* **5**, 582 (1972).
